# Supplementary material for: Locating the gamma-ray emission site in Fermi/LAT blazars. II Multifrequency correlations
Source: arXiv:1511.02654 ancillary file (2015-11-09)
Supplement: Supplementary file 1 [file online_fig1.pdf]

0234+285

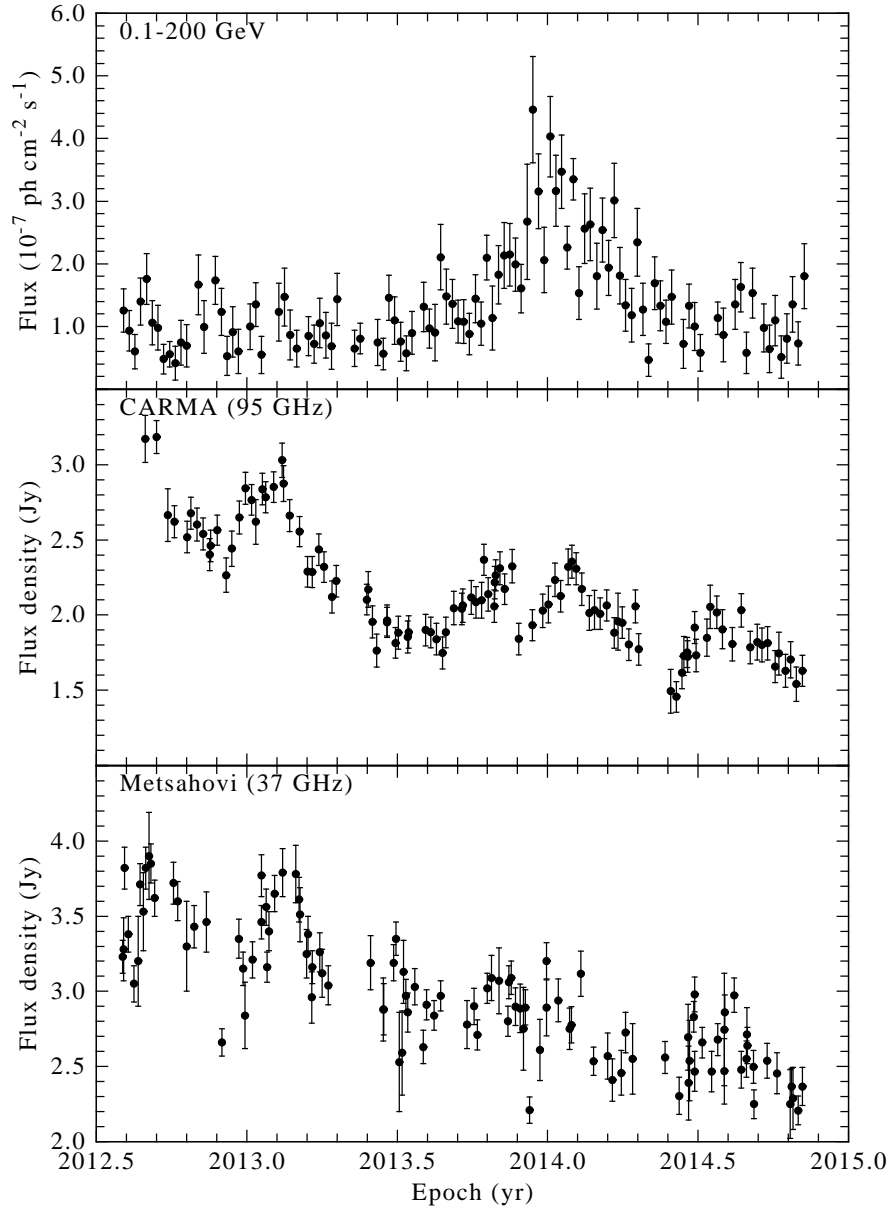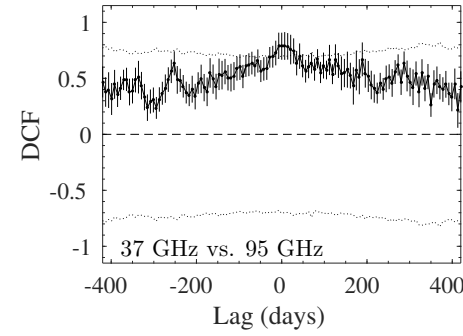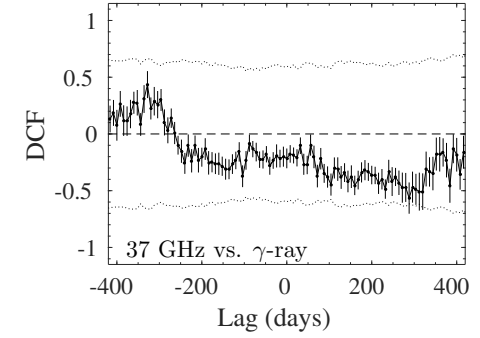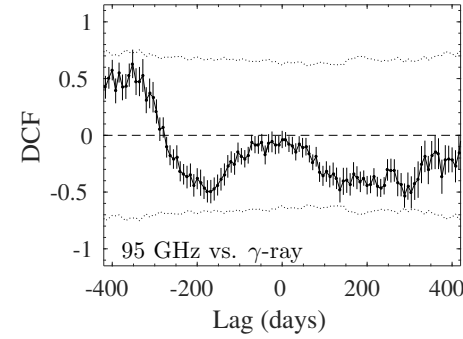

Figure 1.1: Left: Multifrequency light curve of 0234+285. Right: Cross-correlations for all the wavebands. The dotted line in the correlations corresponds to the 99 per cent significance level estimated from simulations.

0235+164

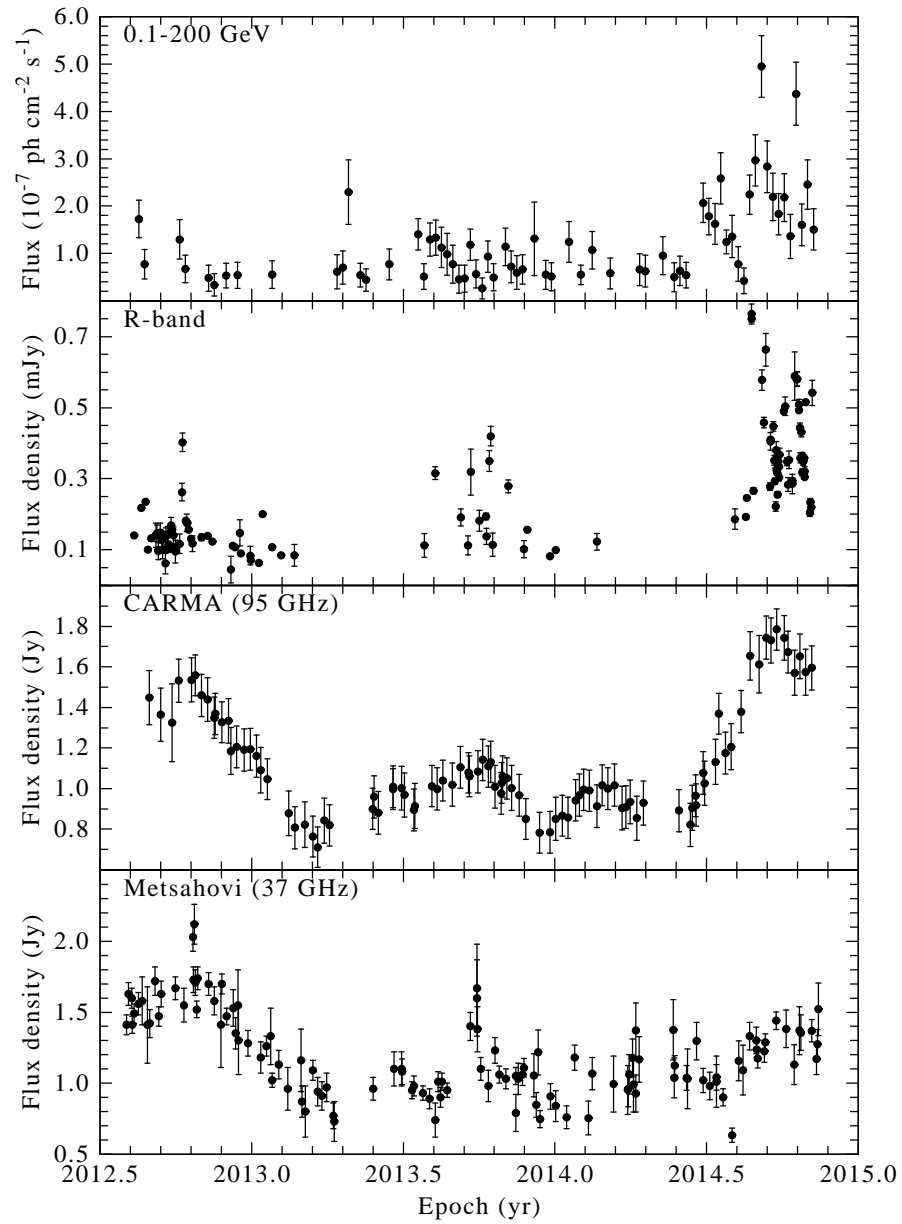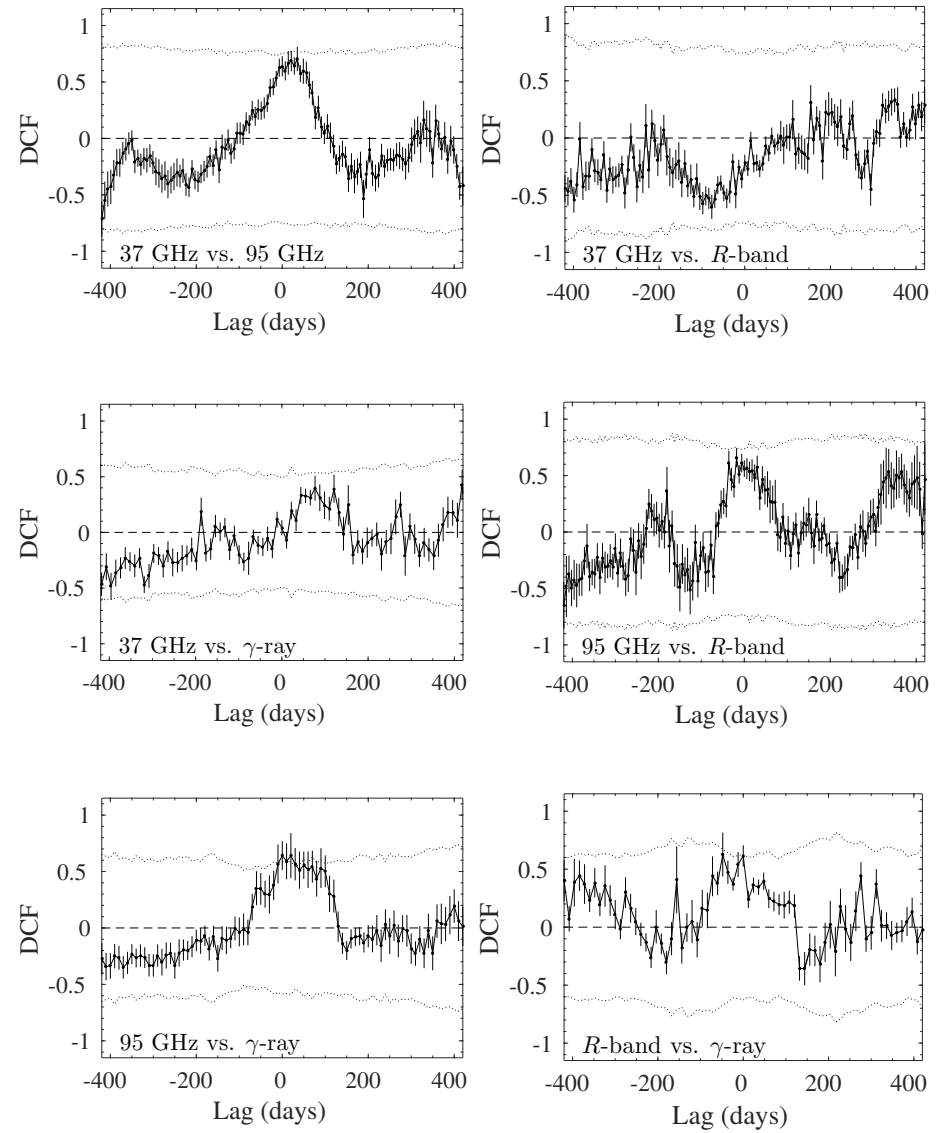

Figure 1.2: 0235+164.

0716+714

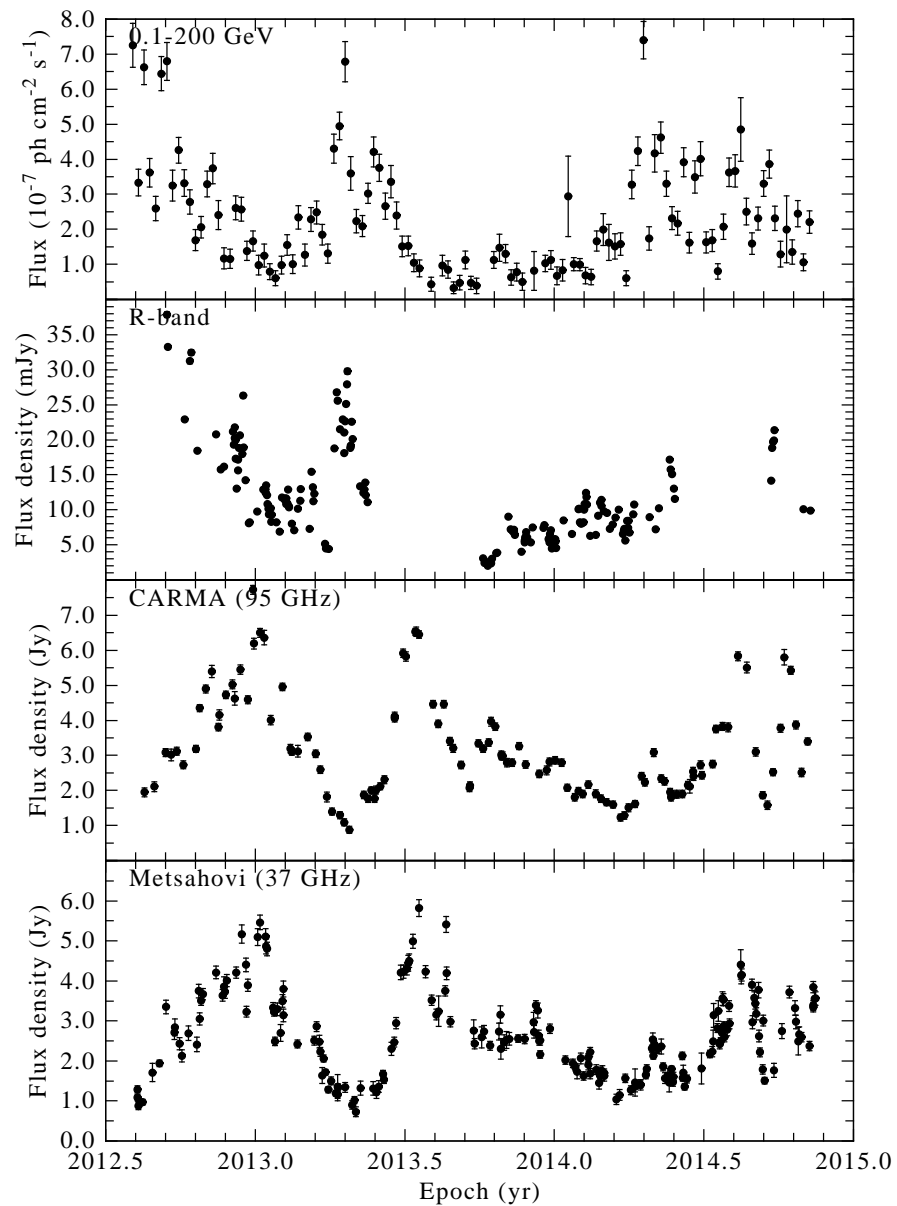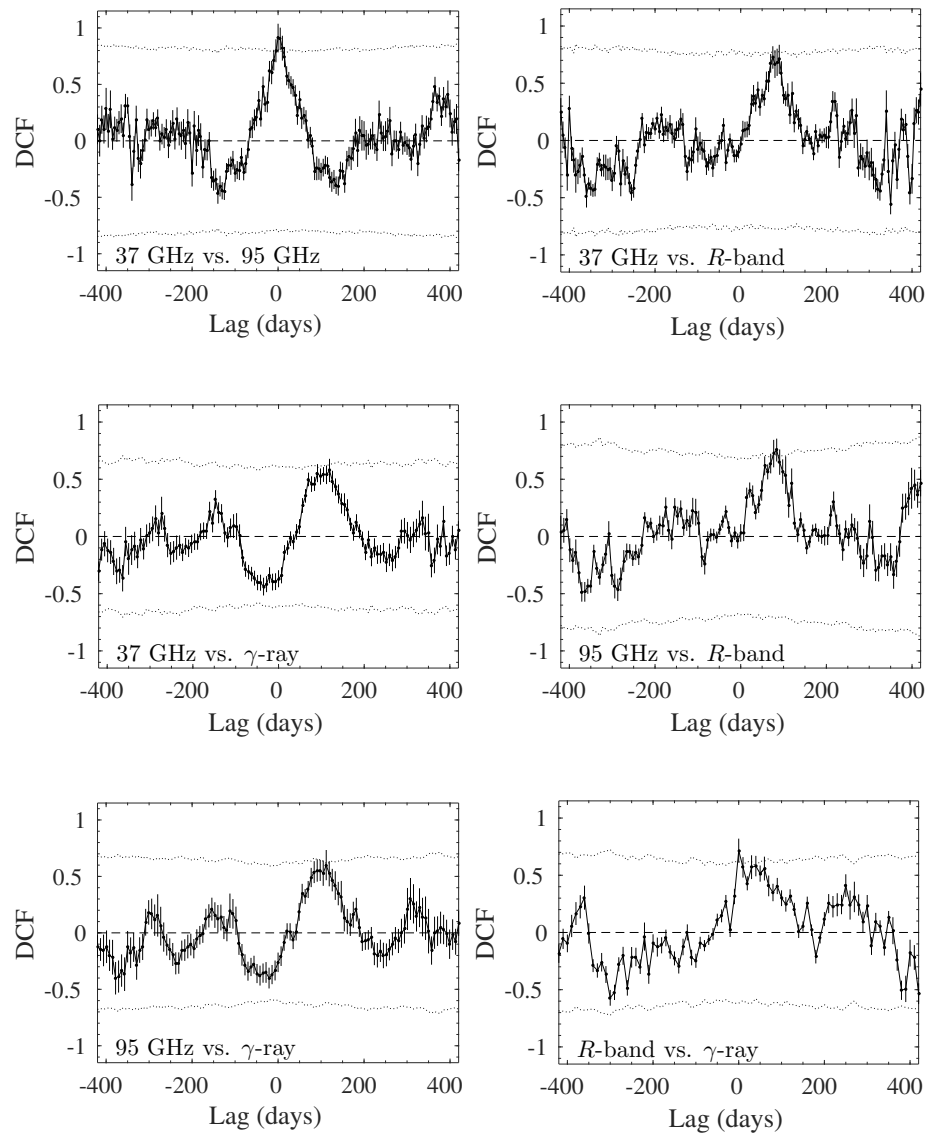

Figure 1.3: 0716+714.

0736+017

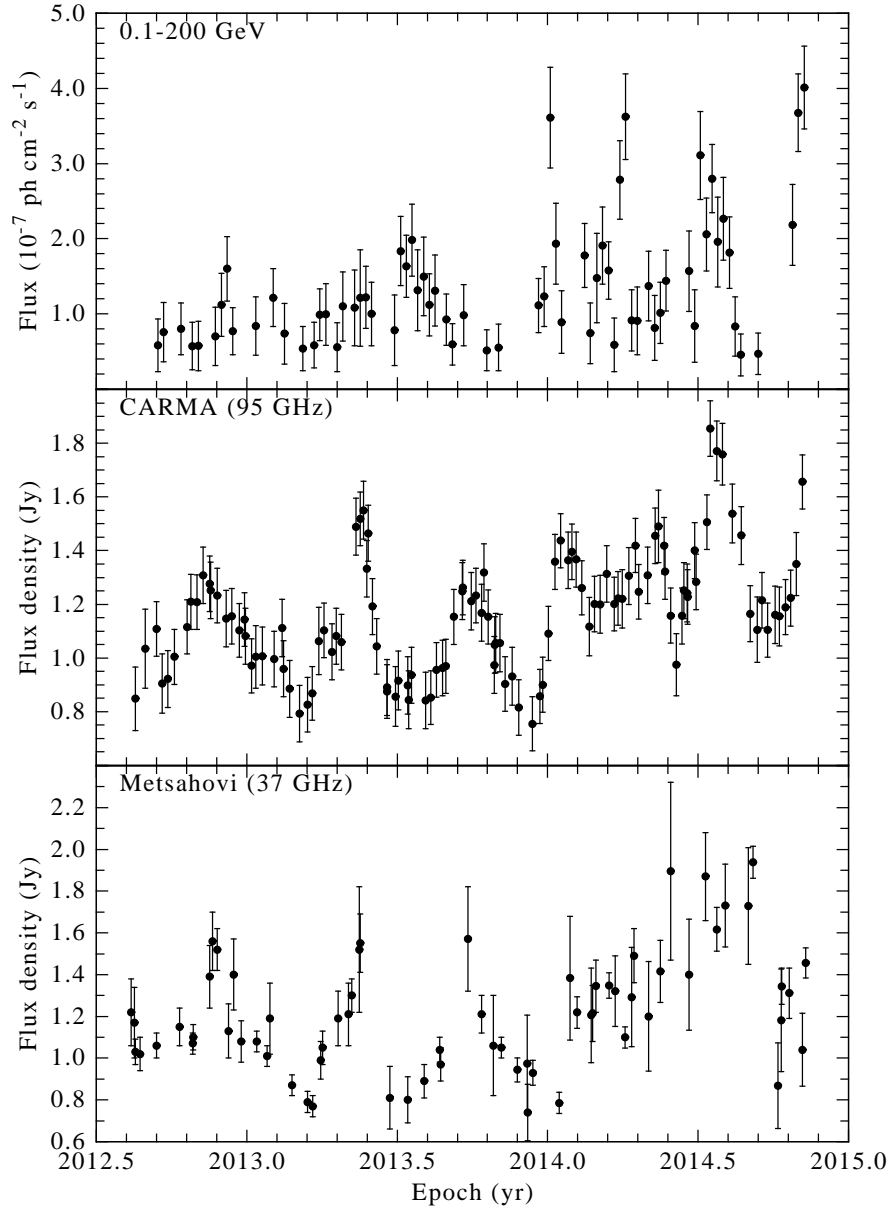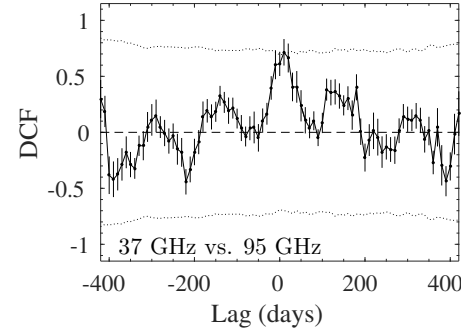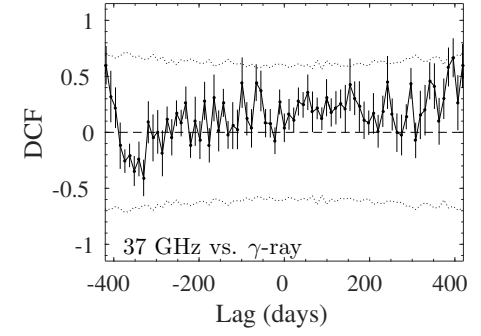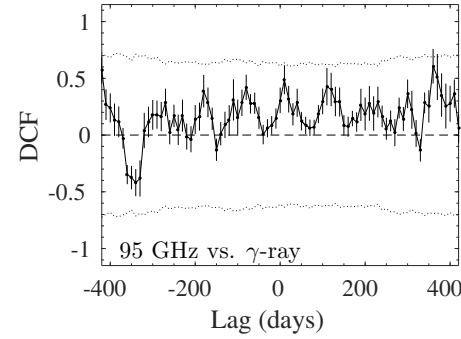

Figure 1.4: 0736+017.

0805-077

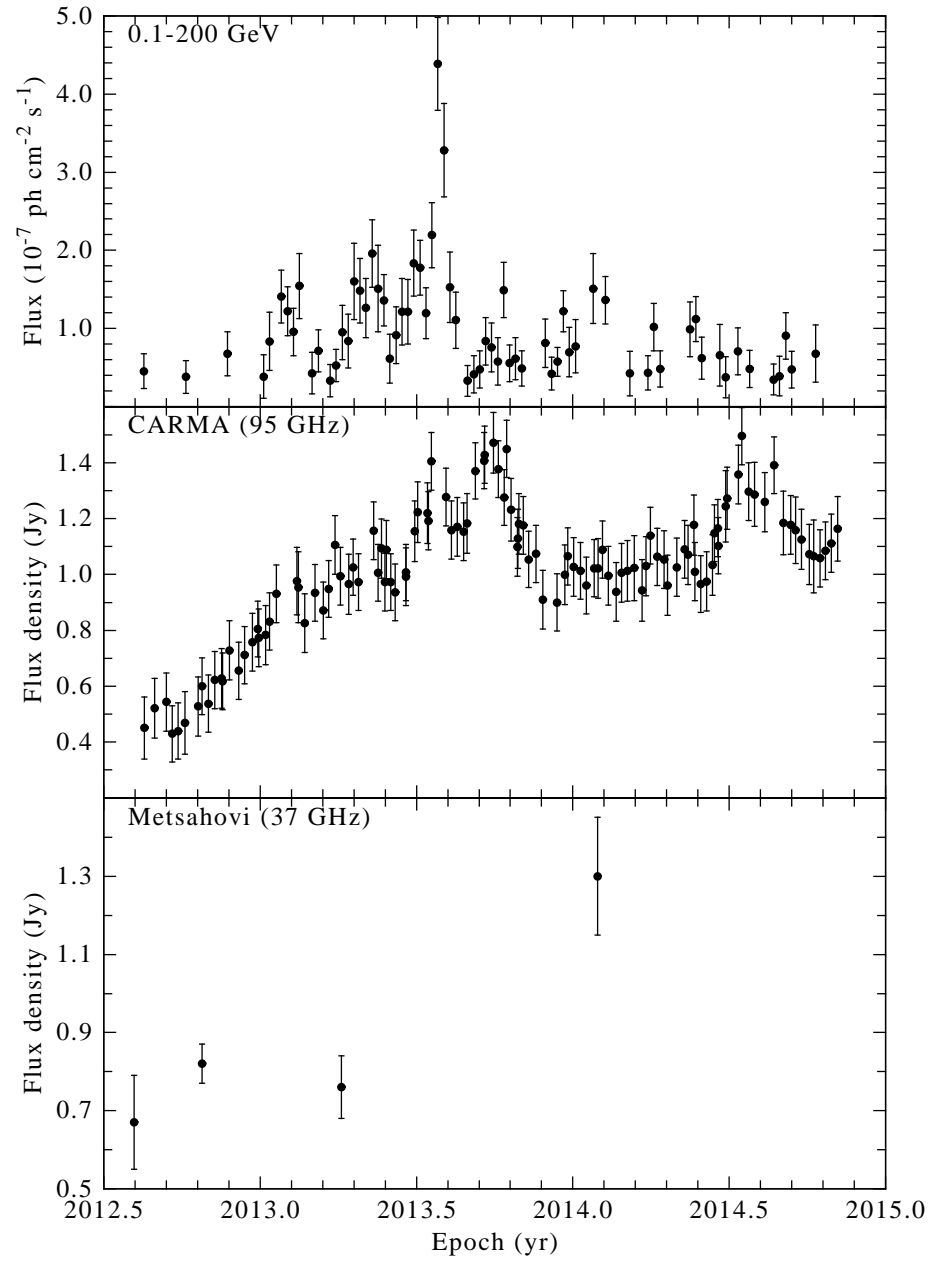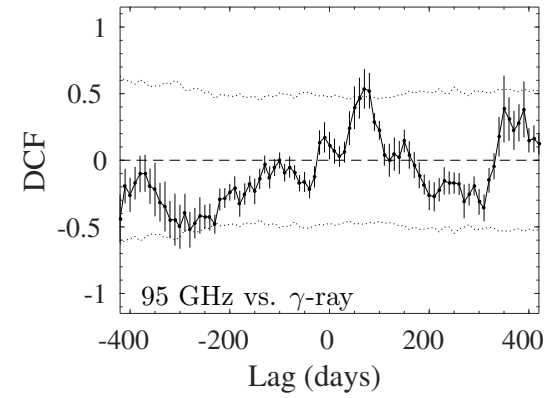

Figure 1.5: 0805-077.

0917+449

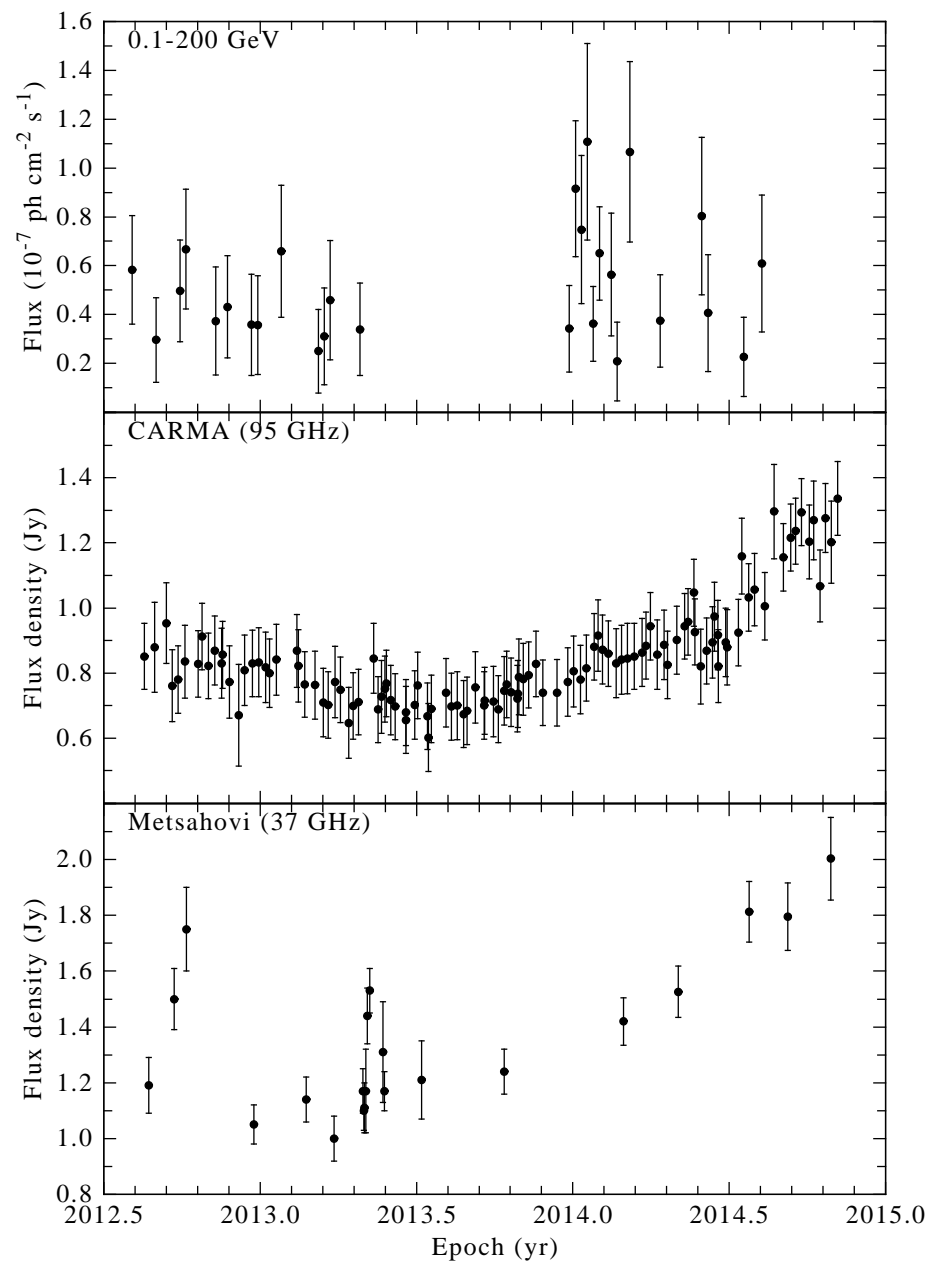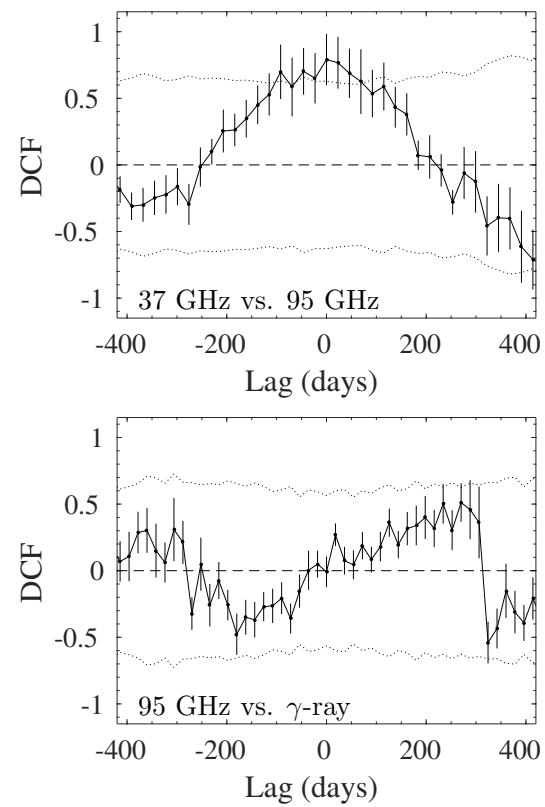

Figure 1.6: 0917+449.

1222+216

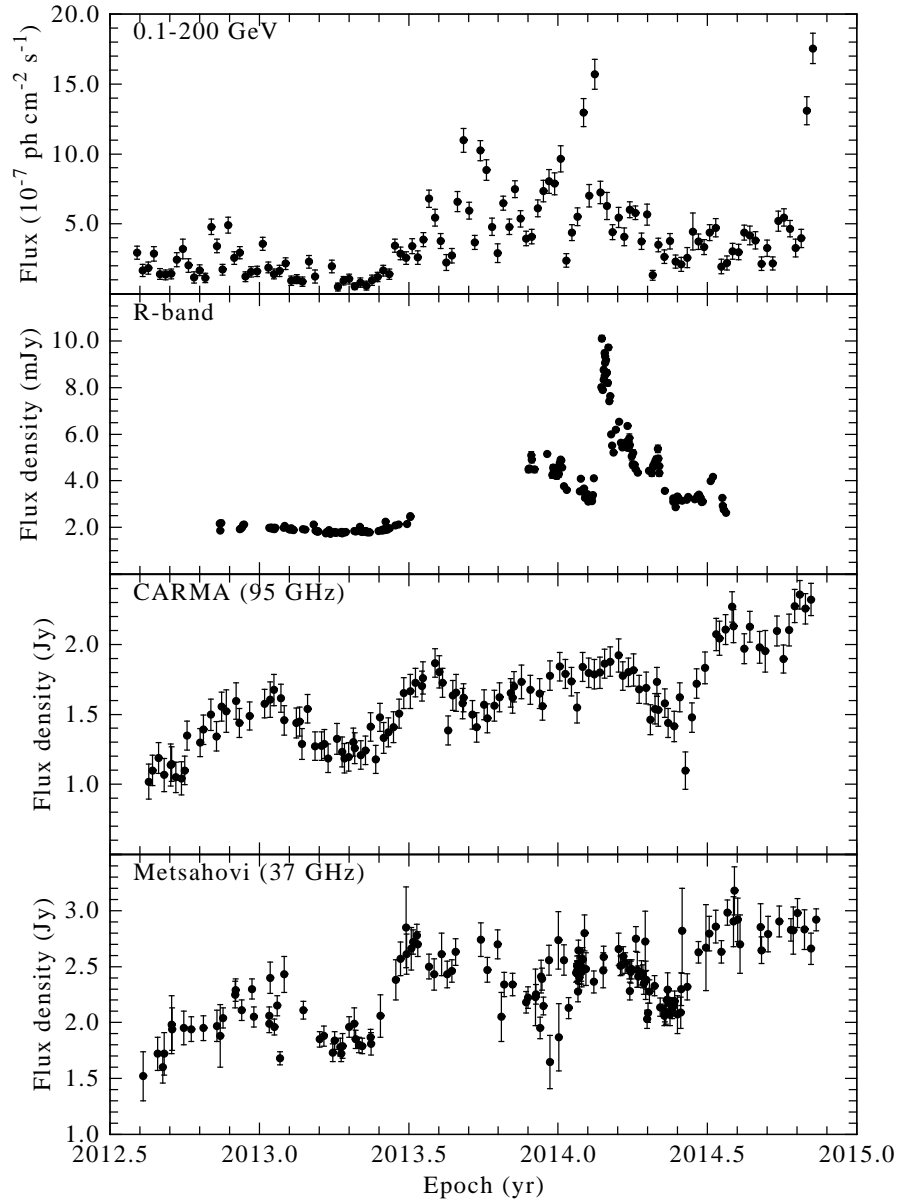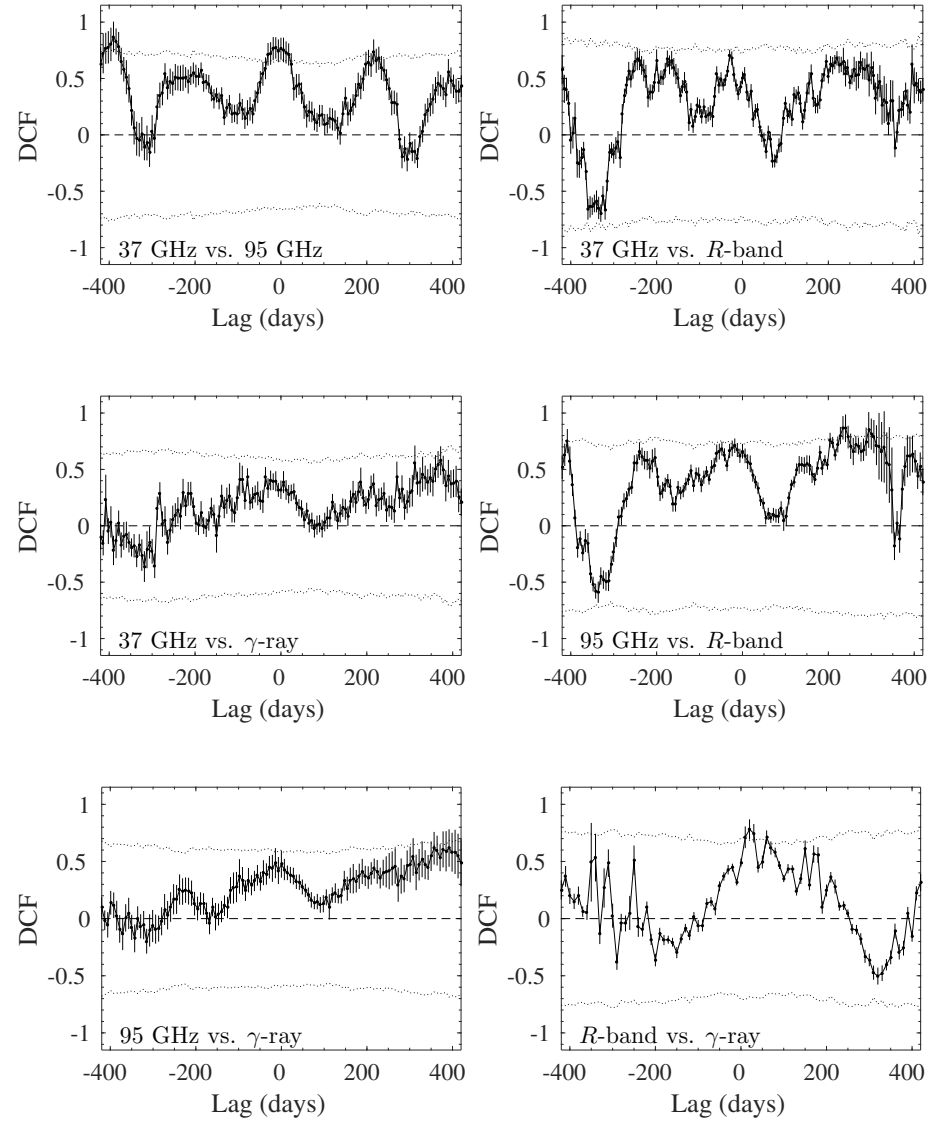

Figure 1.7: 1222+216.

3C273

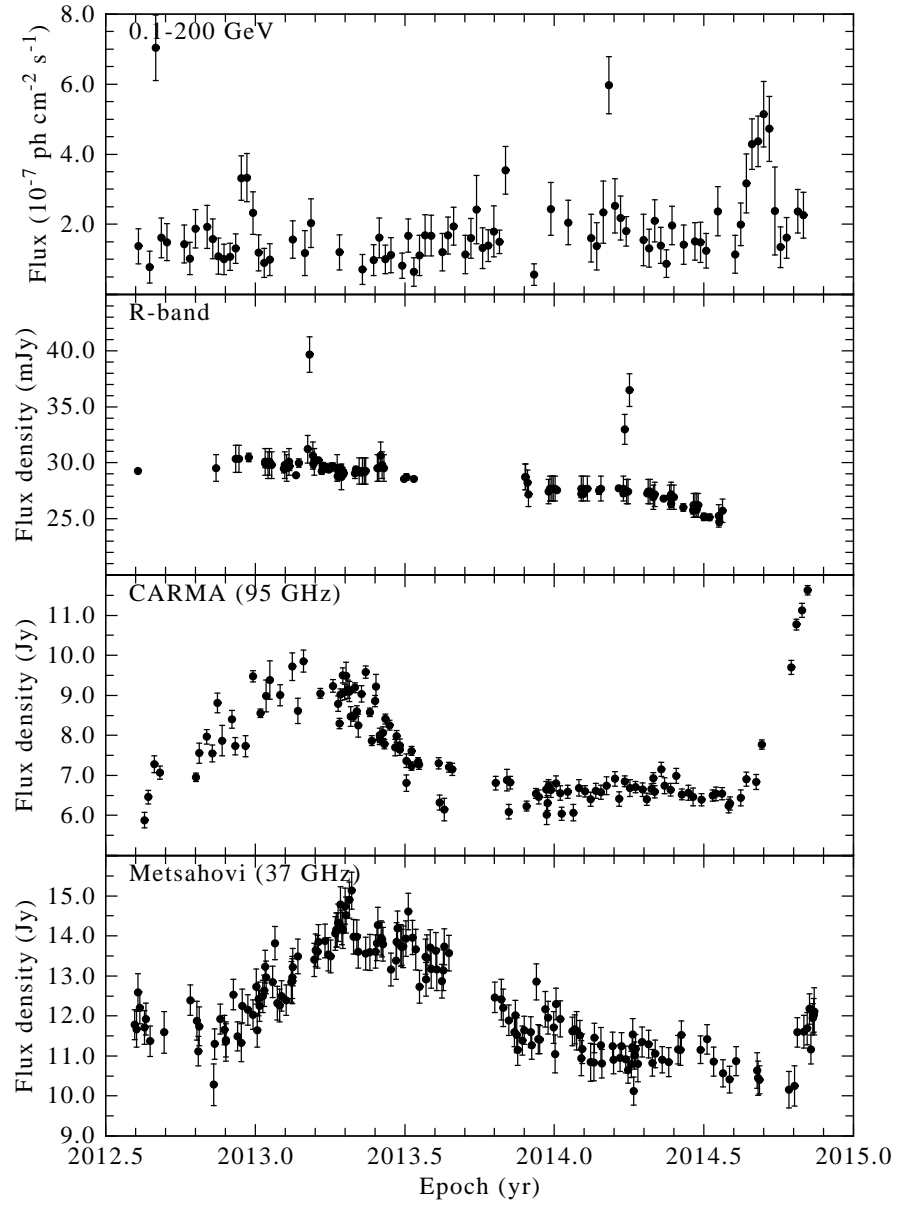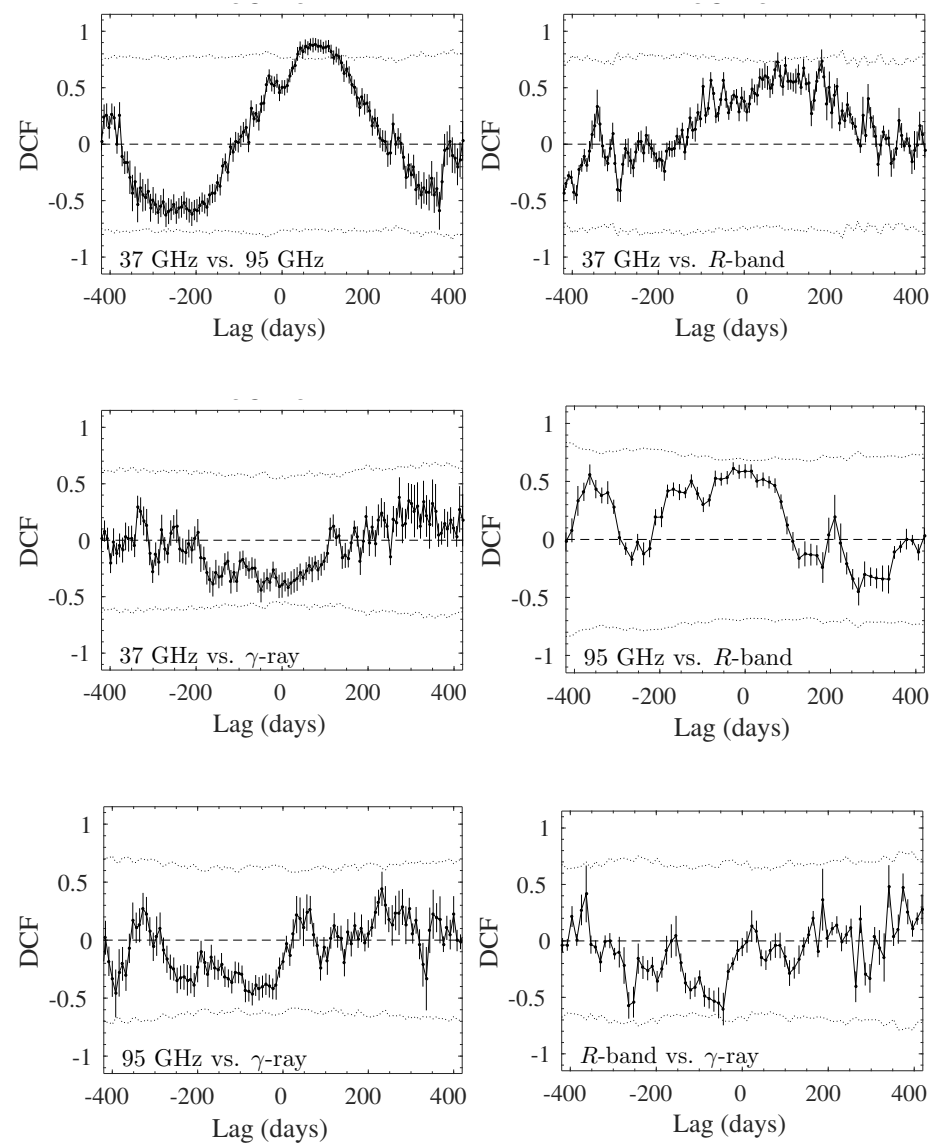

Figure 1.8: 3C 273.



3C279

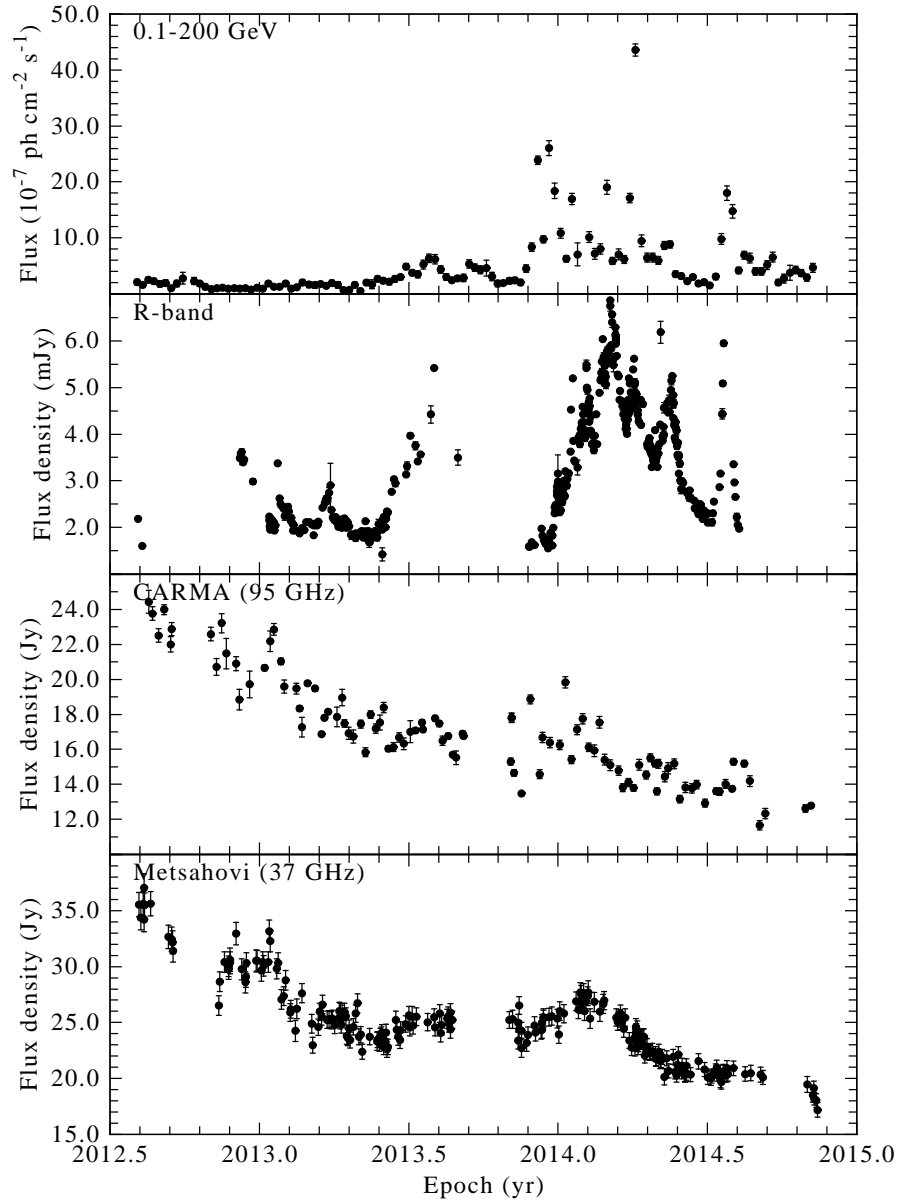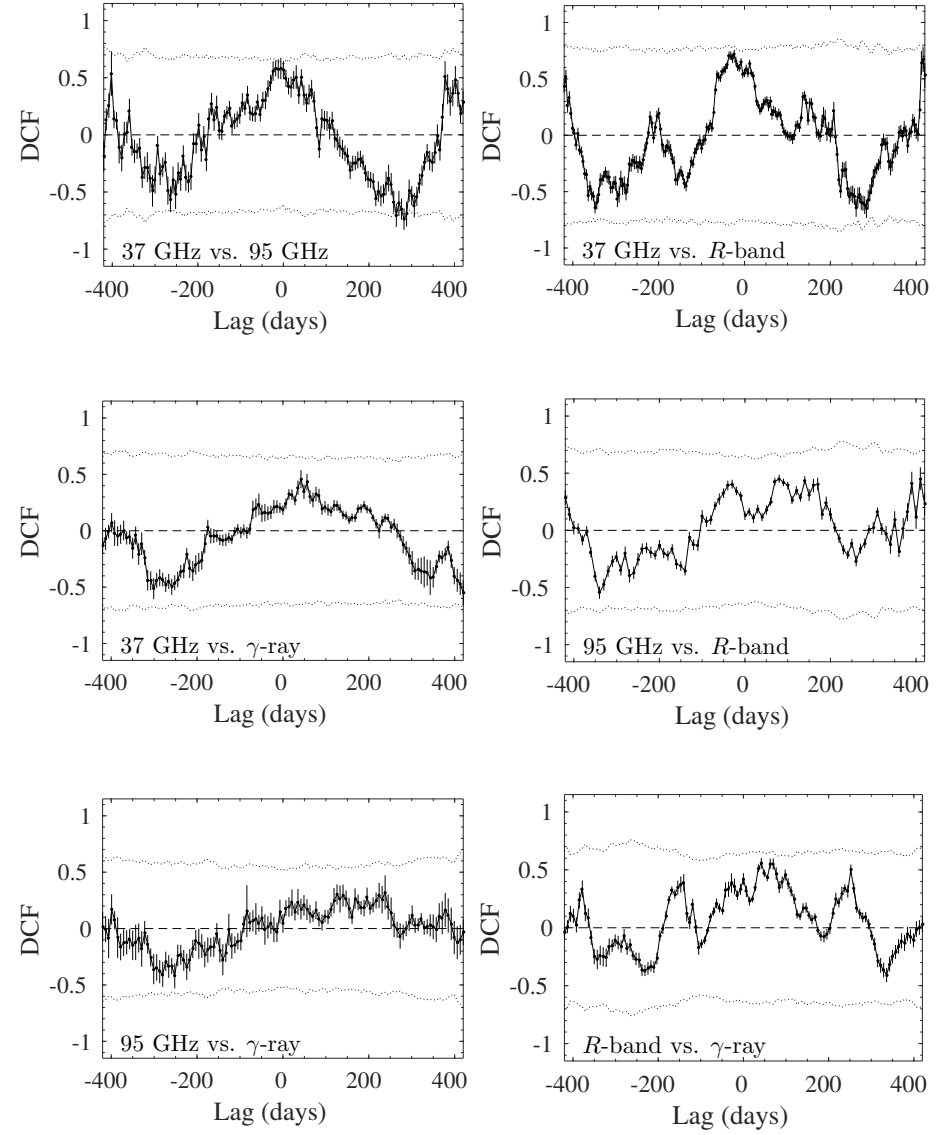

Figure 1.9: 3C 279.

1510-089

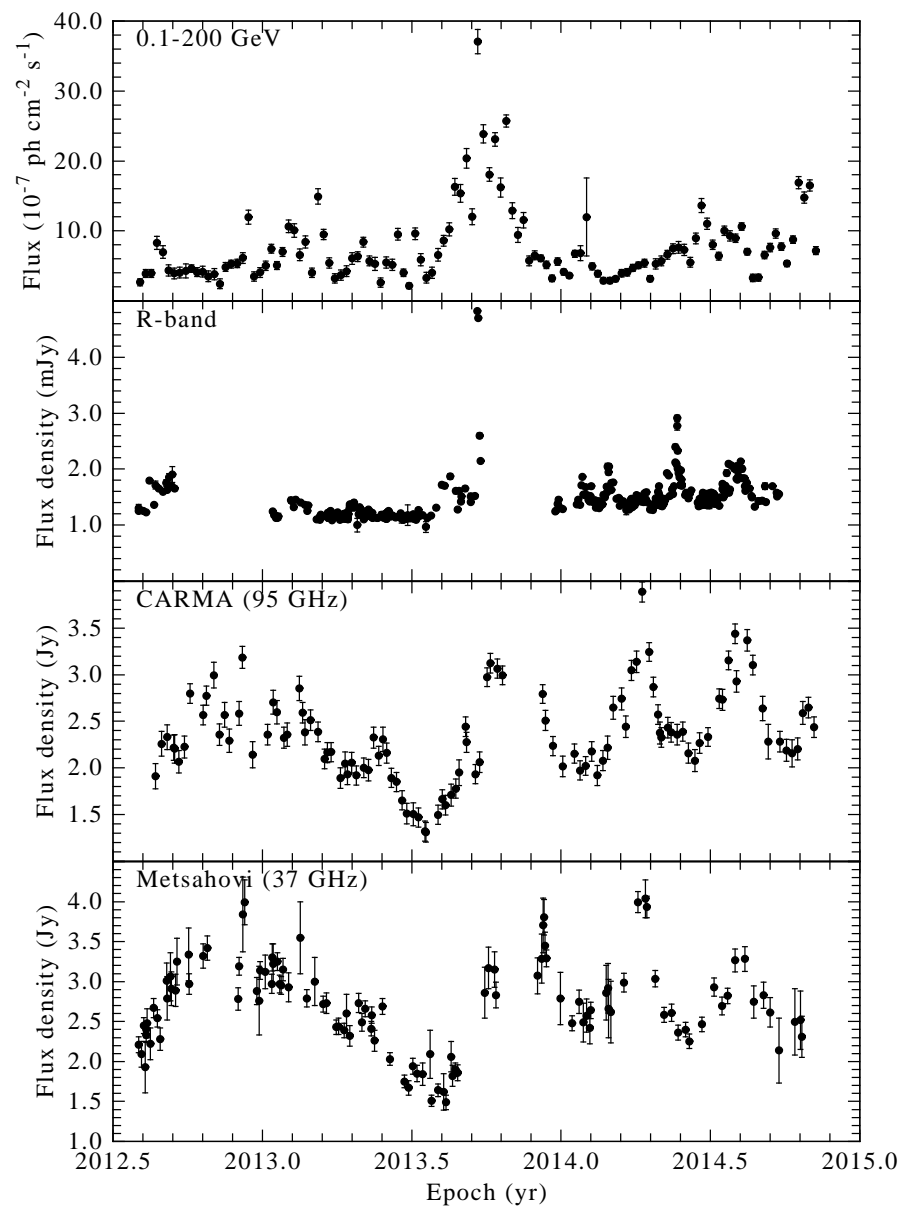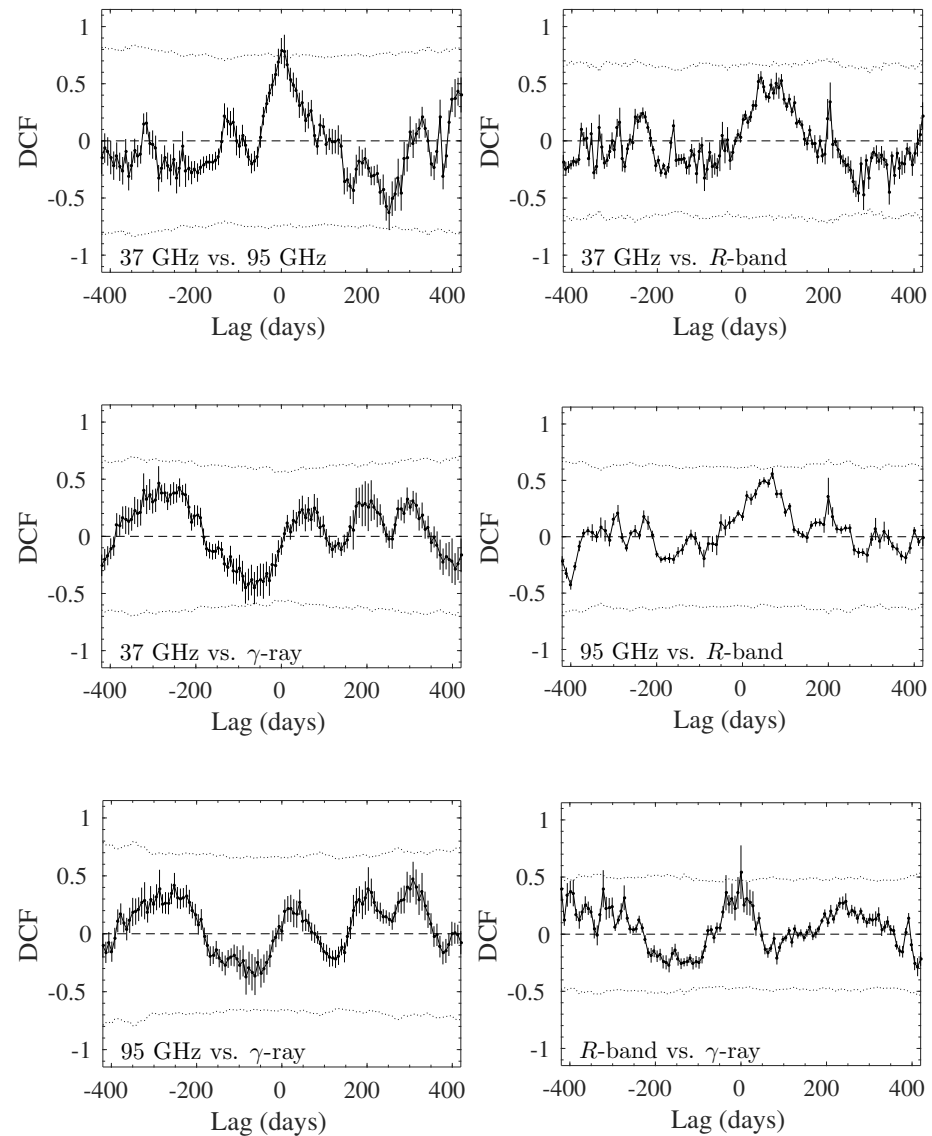

Figure 1.10: 1510–089.

2141+175

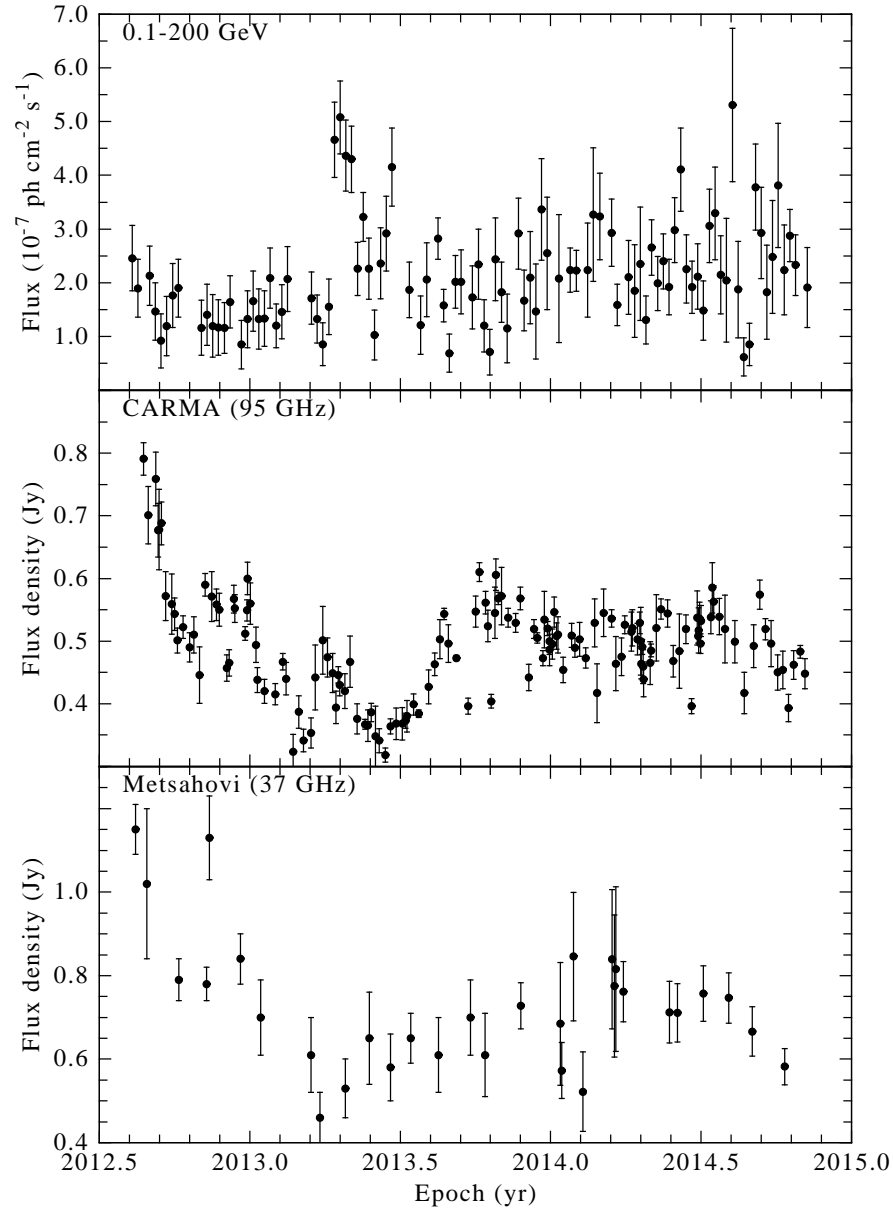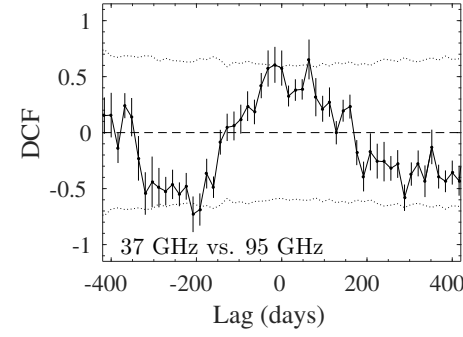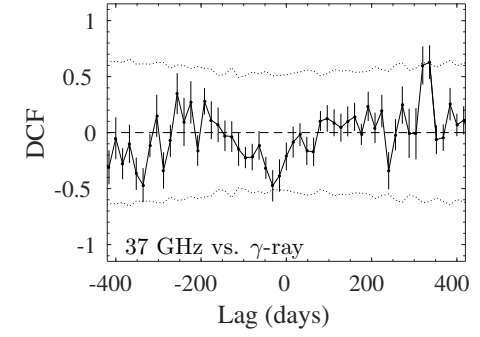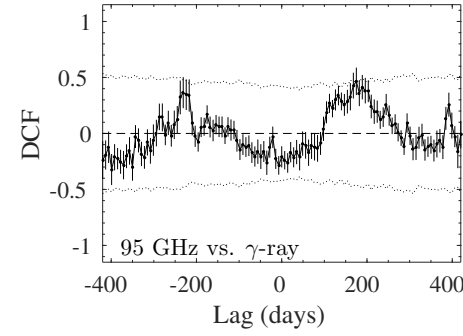

Figure 1.11: 2141+175.

# BLLAC

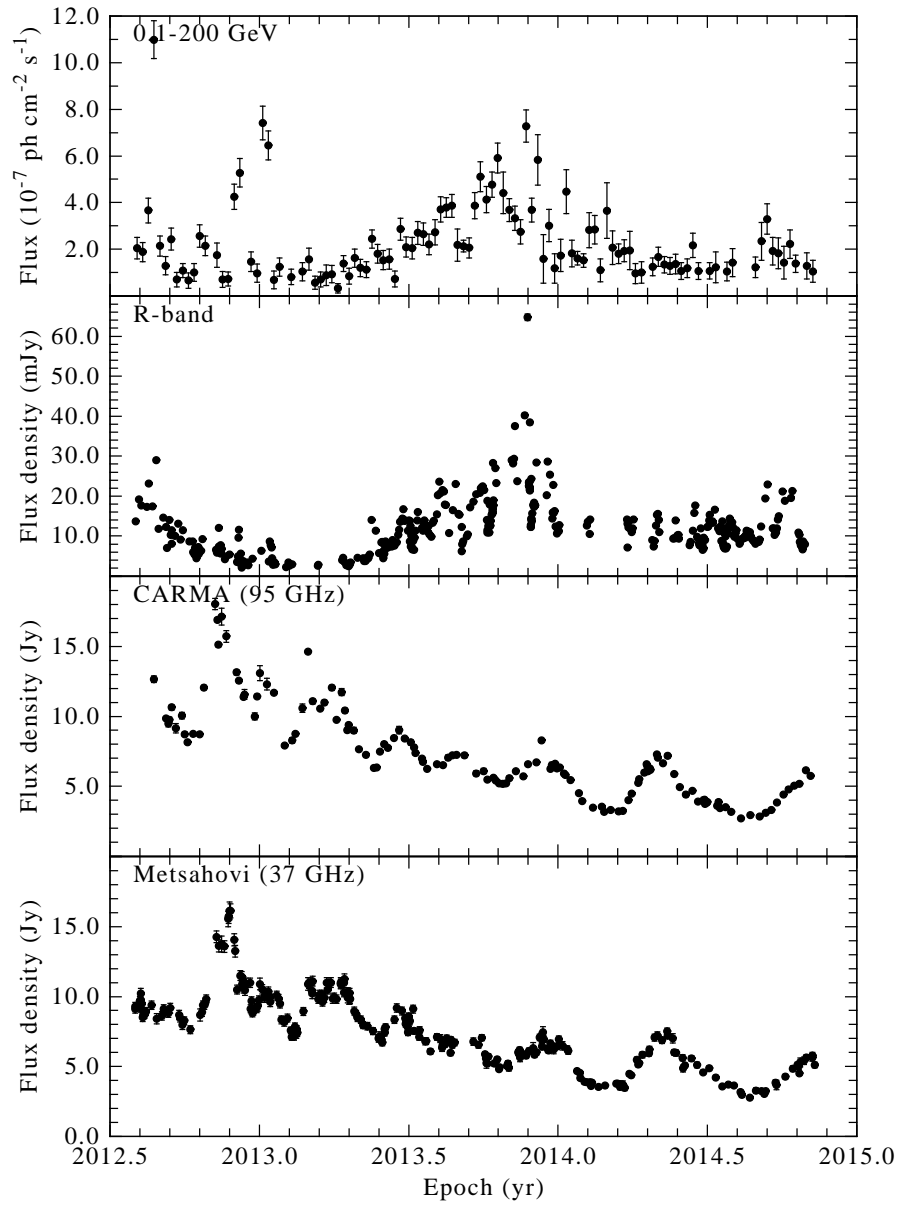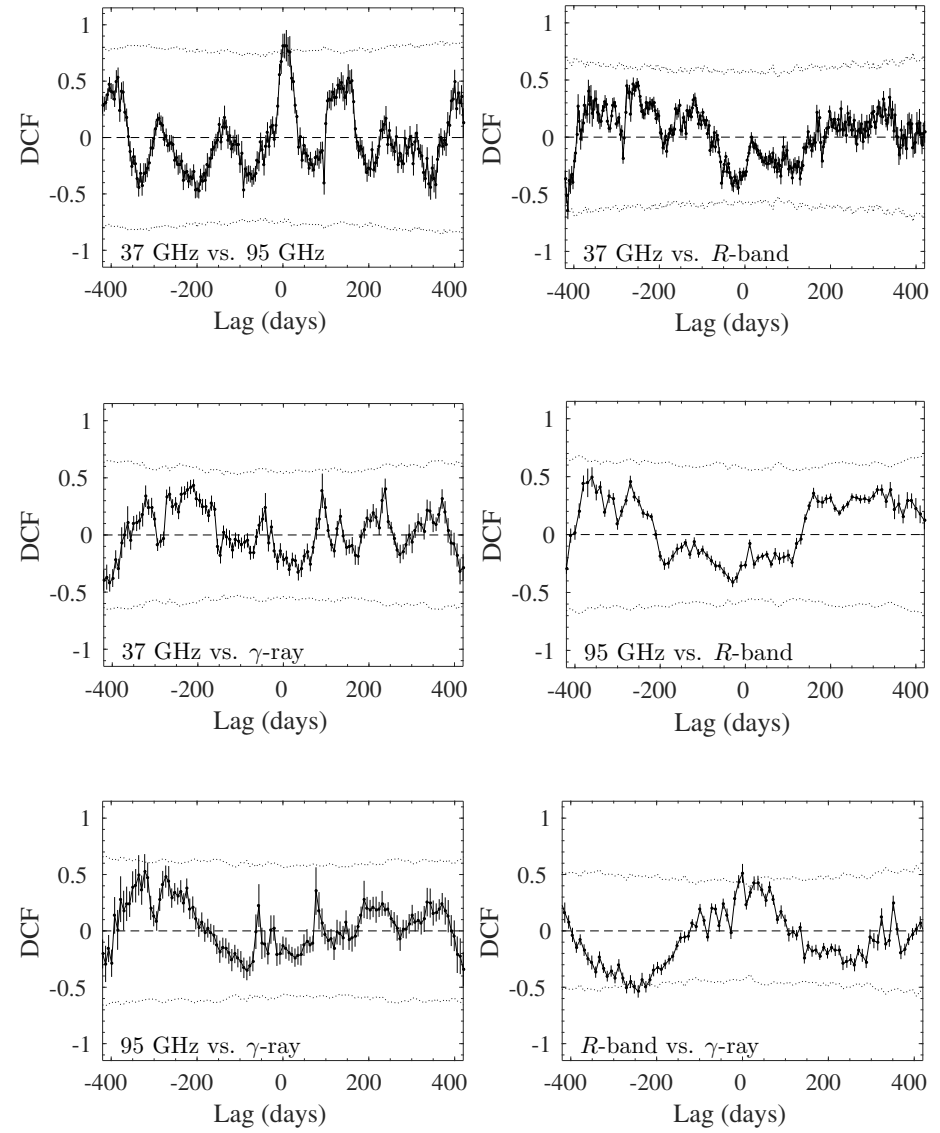

Figure 1.12: BL Lac.

2201+171

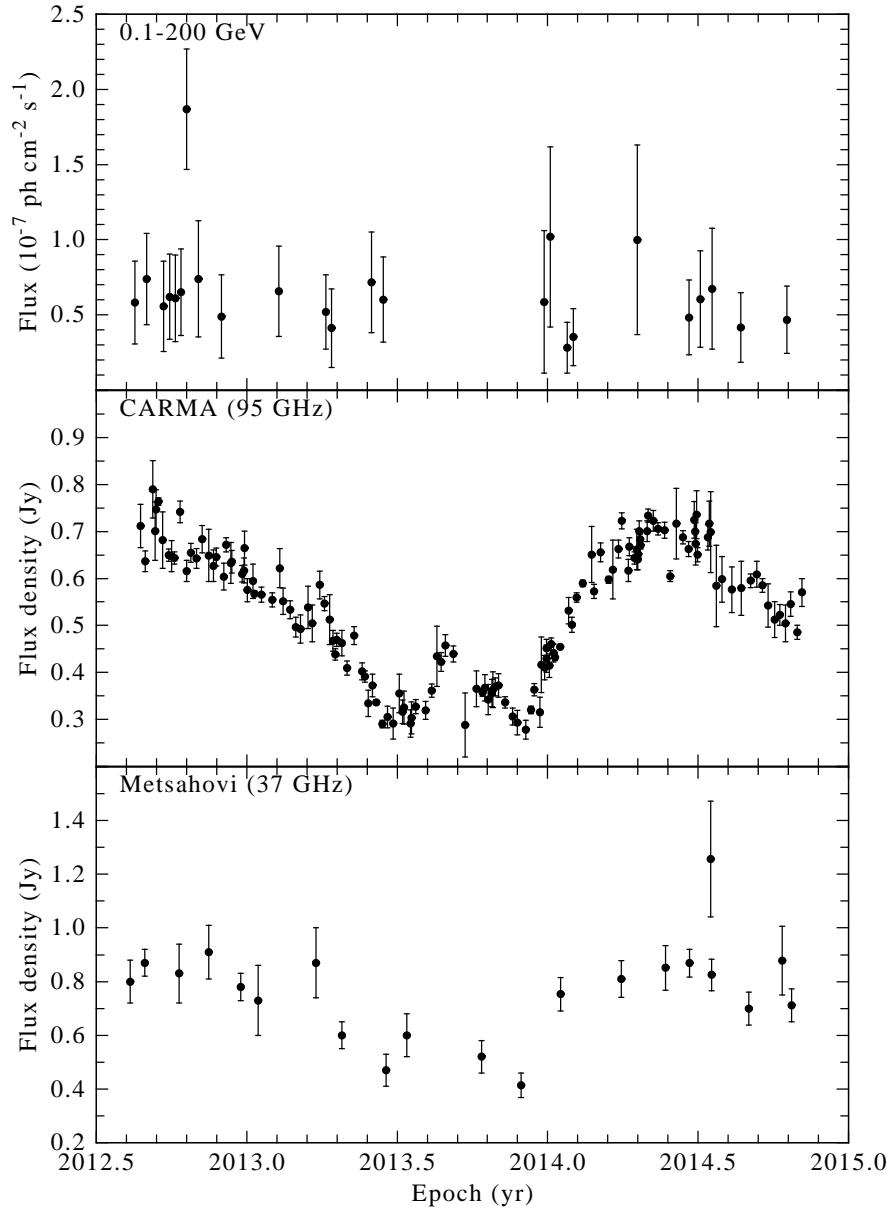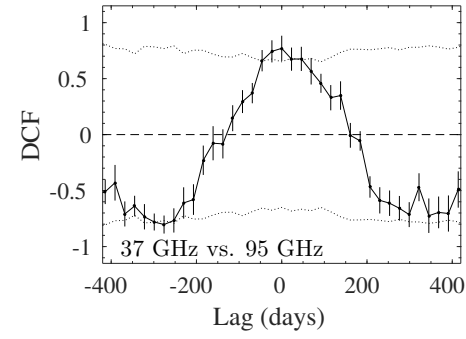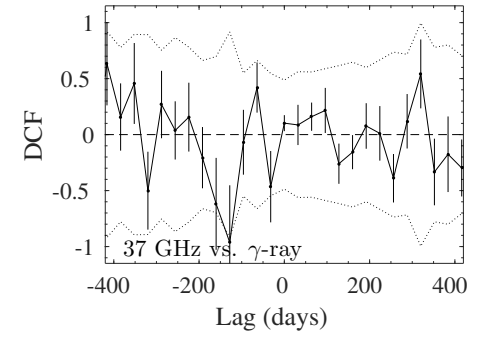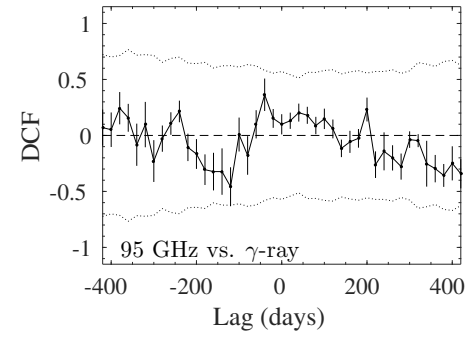

Figure 1.13: 2201+171.

2230+114

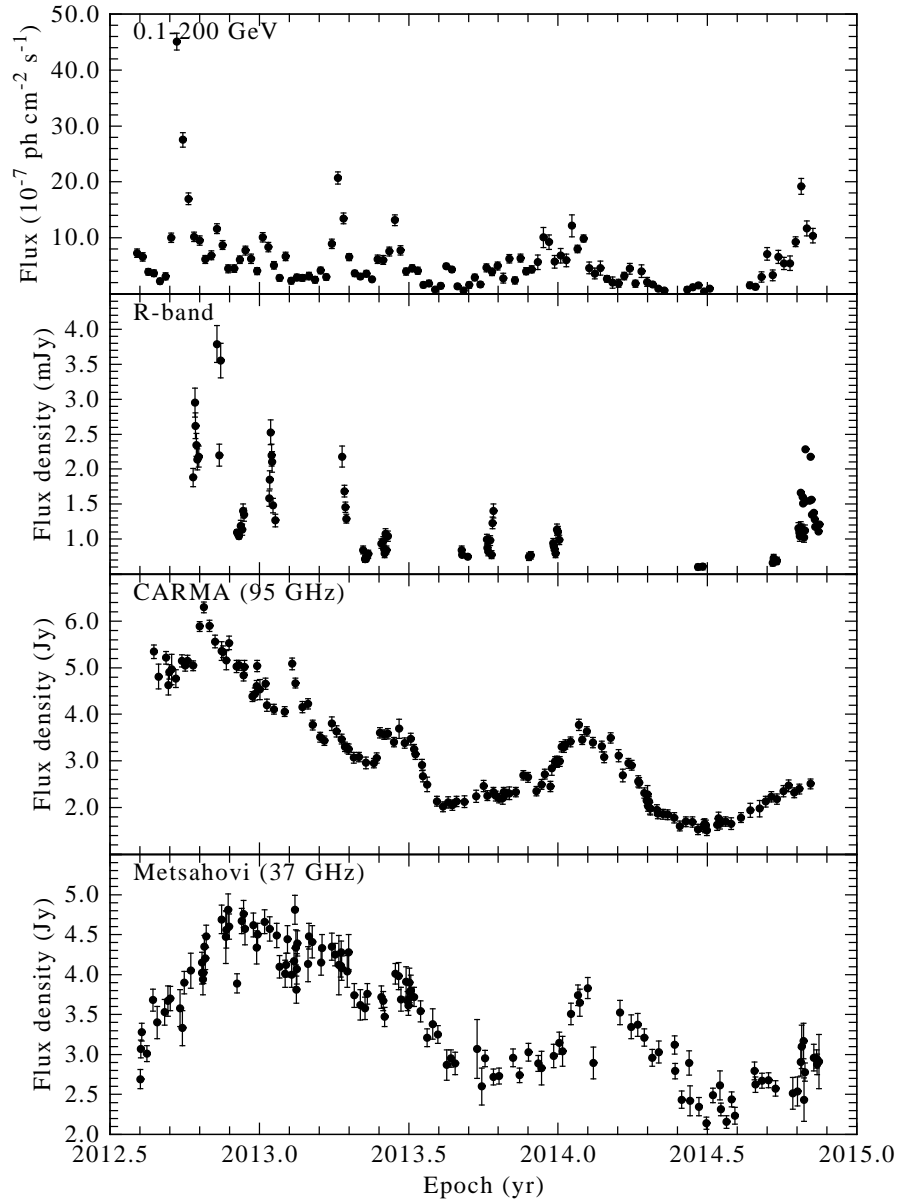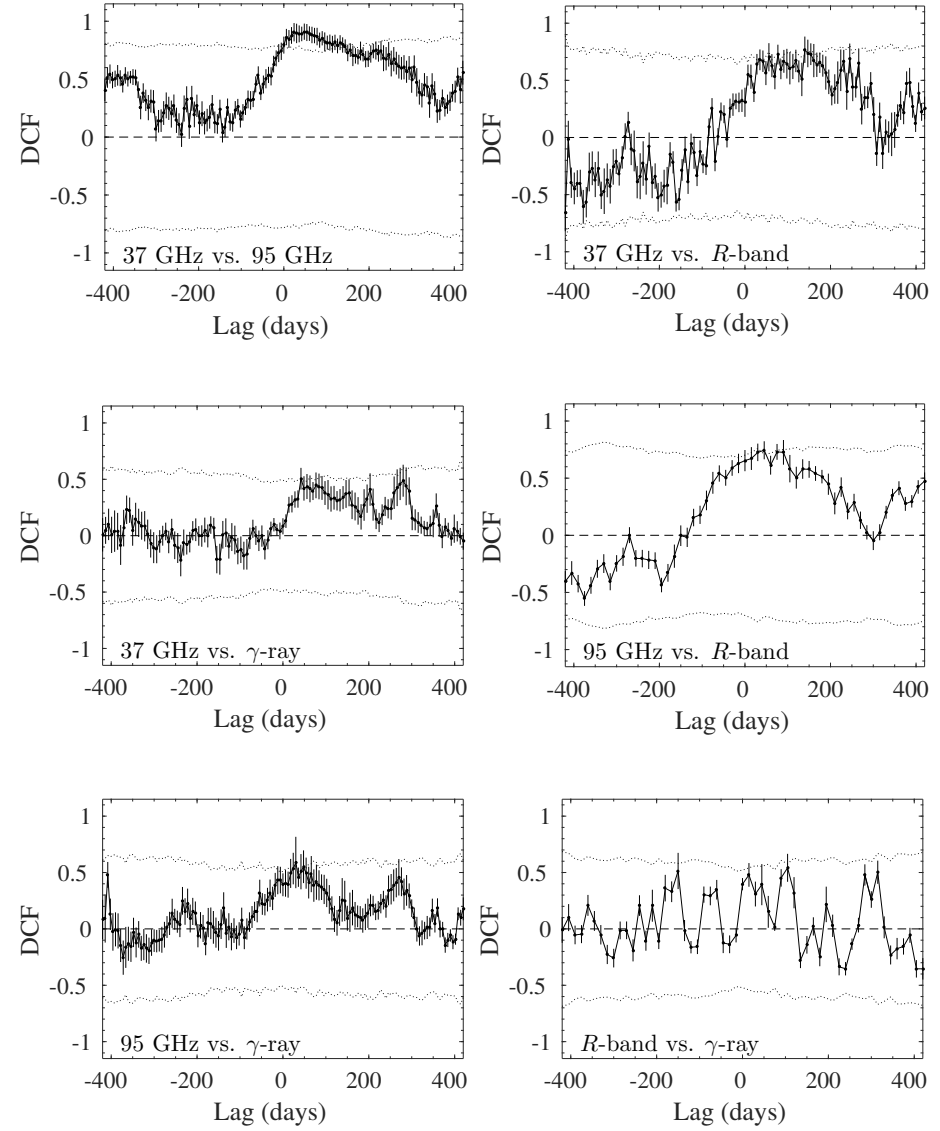

Figure 1.14: 2230+114.

3C454.3

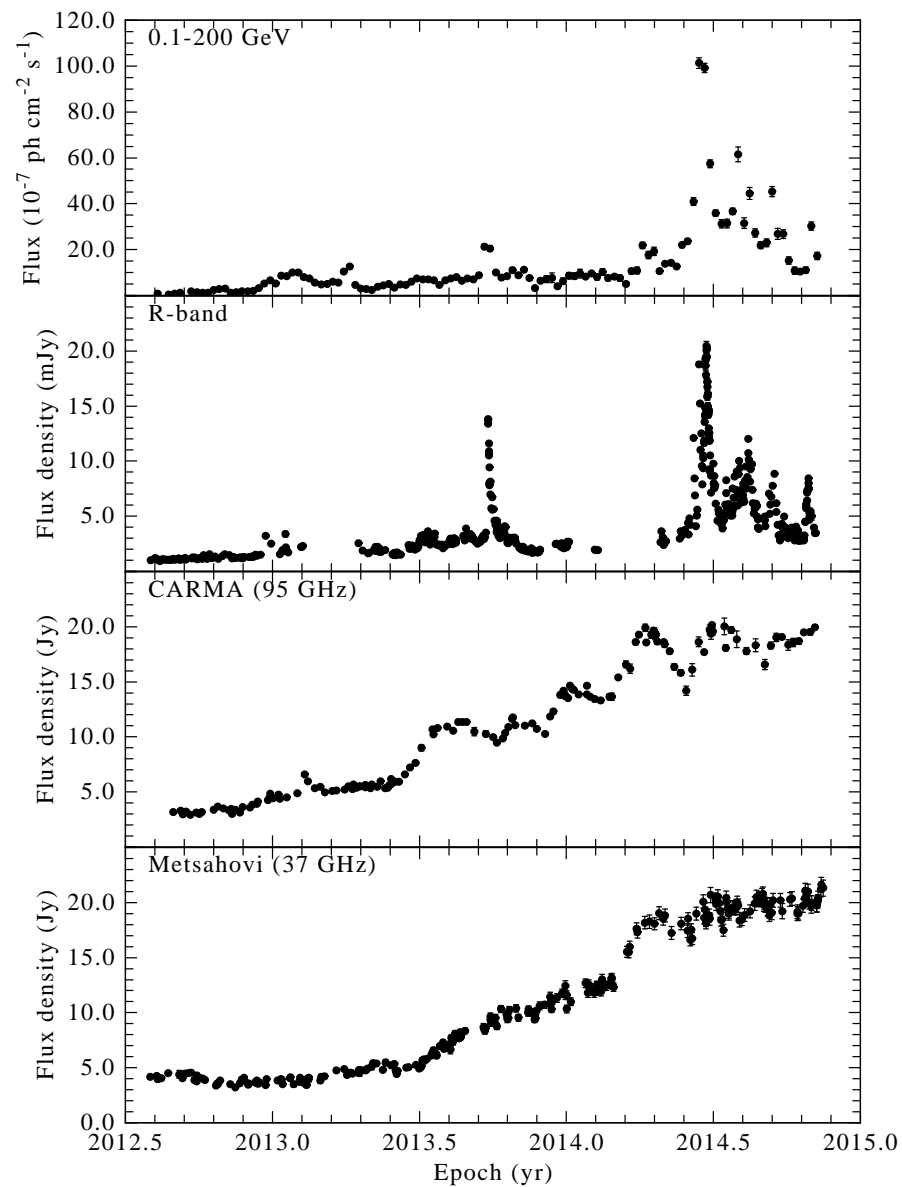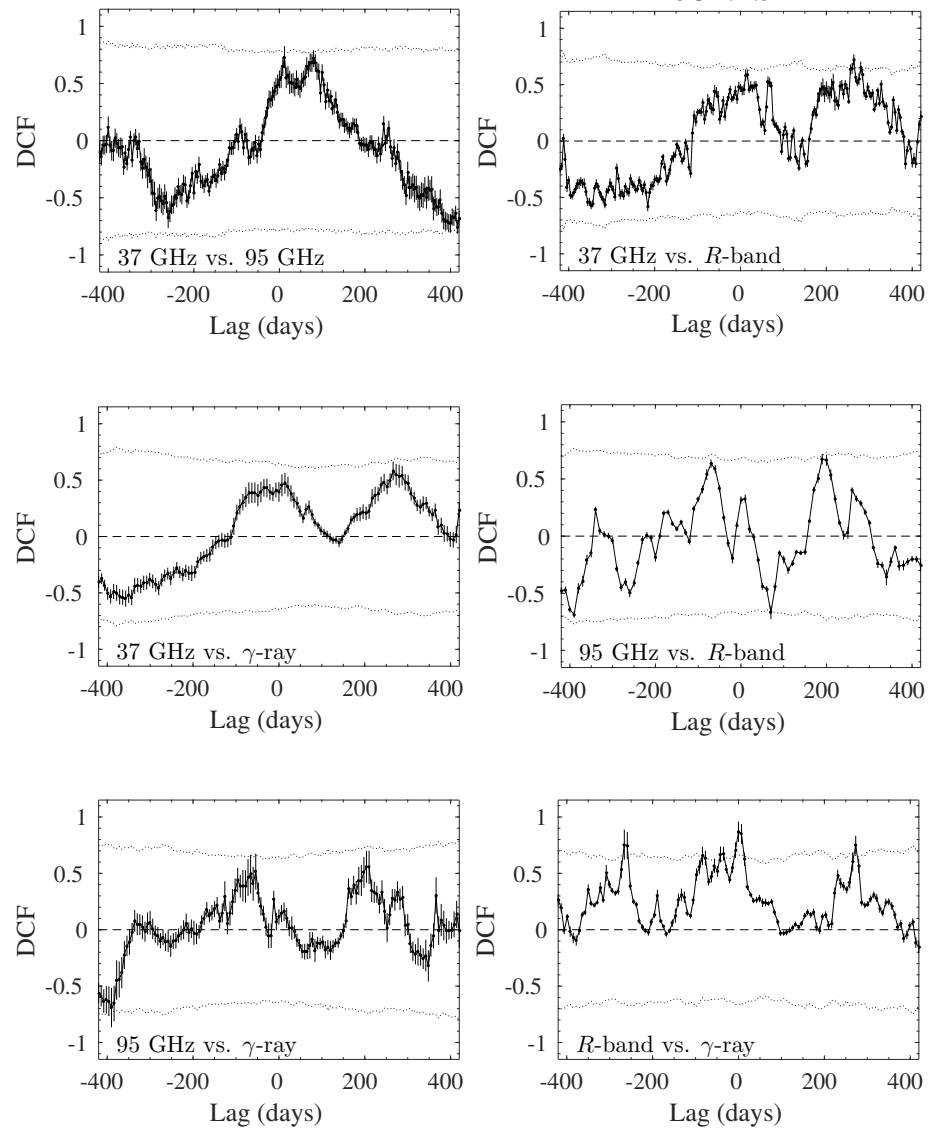

Figure 1.15: 3C 454.3.
